# Supplementary material for: Liquids more stable than crystals
Source: arXiv:1307.1842 ancillary file (2013-07-07)
Supplement: Supplementary file 1 [file supp.pdf]

# Liquids more stable than crystals: Supplementary Information

Frank Smallenburg and Francesco Sciortino
*Department of Physics, Sapienza, Universitá di Roma, Piazzale Aldo Moro 2, I-00185, Roma, Italy*

## IMPLEMENTATION OF THE MODEL

In the model used in this paper, two patches can (but do not have to) bond whenever their bonding volumes overlap, as determined via the normal Kern-Frenkel criterium[1]. The energy decrease associated with forming a bond is given by $\epsilon$. Thus, for a patch with only one bonding candidate (i.e. an overlapping patch not involved in a bond with any other particle) a bond exists with a finite probability governed by the Boltzmann factor:

$$\frac{P(\text{bonded})}{P(\text{unbonded})} = \exp(\beta\epsilon). \tag{1}$$

However, for sufficiently wide patches, a patch may have multiple ($k$) possible bonding partners. In that case, the probability of bonding to each of these candidates is equal, and given by an equilibrium between $k$ possible bonded states (with energy $\epsilon$, and one unbonded state (with energy 0). Hence, the probability $p_B(i)$ of being bonded to any *specific* candidate $i$ ($1 \leq i \leq k$) is given by:

$$p_B(i) = \frac{\exp(\beta\epsilon)}{1 + k\exp(\beta\epsilon)}, \tag{2}$$

and the probability of being unbonded is

$$p_B(0) = \frac{1}{1 + k\exp(\beta\epsilon)}. \tag{3}$$

Technically, this is achieved by generating a random number between zero and one and decide if the bond exists by comparing such number with $p_B(0)$. If the bond exists, a random bonding partner (between one and $k$) is selected.

It should be noted that this still results in an effective interparticle attraction at $\epsilon = 0$: the entropy associated with the option of forming a bond causes states that allow for the formation of bonds to be more likely. At $\epsilon \to -\infty$, this model reduces to hard spheres, since no bonds are formed at all. As a result, this modification of the Kern-Frenkel model does not straightforwardly correspond to the original model even when the patches are so narrow that multiple bonds per patch are prevented by geometric constraints. The model is equivalent to the KF model with an *effective* well depth $\epsilon_{\text{eff}} = k_B T \log(1 + \exp(\beta\epsilon))$. This can be shown as follows. In the original model, the probability ratio between finding the system in a specific point in phase space $\{\mathbf{r}^N, \mathbf{\Omega}^N\}$ with $N_b$ bonds and a different configuration ( with no overlaps) with zero bonds is:

$$\frac{p(N_b)}{p(0)} = \exp(N_b\beta\epsilon). \tag{4}$$

In the modified model, this ratio consists of all possible ways of bonding the system, which includes 1 way where no bonds are made, $N_b$ ways where 1 bond is made, and so on:

$$\begin{aligned} \frac{p(N_b)}{p(0)} &= \sum_{n=0}^{N_b} \binom{n}{N_b} \exp(n\beta\epsilon) && (5)\\ &= (1 + \exp(\beta\epsilon))^{N_b} && (6)\\ &= \exp(N_b\beta\epsilon_{\text{eff}}) && (7) \end{aligned}$$

Thus, in the case where every patch can only have one bonding candidate, the partition function of the modified model can be rewritten as one for the original Kern-Frenkel model, but with $\epsilon$ replaced by $\epsilon_{\text{eff}}$. For large $\epsilon$, $\epsilon_{\text{eff}} \simeq \epsilon$, and $\epsilon_{\text{eff}} \to 0$ for $\epsilon \to -\infty$.

In Monte Carlo simulations, implementation of the single-bond Kern-Frenkel model is straightforward. To make and break bonds, a Monte Carlo move is introduced that selects a random patch on a random particle, and determines which patches on other particles are available for bonding (i.e. overlapping and currently unbonded). Then, the patch is chosen to be either bonded to one of these bonding candidates (if any) or to be unbonded, based on equations (2) and (3). Note that the original bonding state of the patch is not taken into account.

## EVENT-DRIVEN MOLECULAR DYNAMICS

We use Event-driven Molecular Dynamics (EDMD) simulations for calculating the equations of state and potential energies required for thermodynamic integration, and to investigate the dynamics of the low-temperature liquid phase. EDMD simulations are based on the prediction of discrete interactions between particles, such as collisions, or square-well interactions. Since no forces act on the particles except during these instantaneous events, movement of the particles between events is simply Newtonian free motion: the center of mass $\mathbf{r}_i$ moves in a straight line at constant velocity $\mathbf{v}_i$, and the particle rotates with a constant angular momentum $\mathbf{L}_i$. In the case of spheres, the moment of inertia tensor $\mathbf{I}$ is diagonal, with $I_{xx} = I_{yy} = I_{zz} = I$, so that the angular momentum is simply proportional to the angular velocity ($\mathbf{L}_i = I\omega_i$). Predicted collisions are stored in

a binary tree, along with events for updating the cell list and performing measurements. During every step of the simulation, the first event in the event tree is handled, new collisions are predicted, and the event tree is updated[2]. In the EDMD simulations we use here, we employ a cell list to increase the efficiency of checking for possible collisions.

### Event prediction

In EDMD simulations of patchy particles modeled by the (original) Kern-Frenkel model, hard-core collisions between the particles can be predicted analytically. However, numerical algorithms are required to predict interactions via the potential well. Our goal here is to predict the next time two particles start or stop interactions, given their positions, velocities, and angular velocities. The prediction of this event happens in several steps. When first examining a pair of particles, we determine a time interval in which patch interactions might take place, based only on the positions (not orientations) of the particles. As this is entirely based on collisions between spherical regions, this step can be done analytically.

1. Analytically predict the time $t_{\text{min}}$ when the center-to-center distance between the two particles is small enough to allow for the patches to interact ($r < \sigma + \delta$). If this is already the case, set $t_{\text{min}}$ to the current time $t_{\text{current}}$. If the particles will never come close enough to interact, stop looking for interaction events.

2. Analytically predict the collision $t_{\text{max}}$ time between the hard cores of the particles.

3. If no hard-core collision is expected, set $t_{\text{max}}$ to the time when center-to-center distance becomes larger than the maximum interaction range again.

4. Schedule an event to search for a well interaction between the two particles between times $t_{\text{min}}$ and $t_{\text{max}}$, or start the search immediately if $t_{\text{min}} = t_{\text{current}}$.

To search for a well interaction, we have to determine when $\Phi(\mathbf{r_{ij}}, \{\mathbf{p}_i\})$ and $\Phi(\mathbf{r_{ji}}, \{\mathbf{p}_j\})$ switch from 0 to 1 or vice versa, where both the distance vector $\mathbf{r_{ij}} = -\mathbf{r_{ji}}$ between the particles and the orientations of the patches $\{\mathbf{p}_i\}$ and $\{\mathbf{p}_j\}$ are functions of time. To do this, we define a function $\phi(\mathbf{r_{ij}}, \{\mathbf{p}_i\})$ that represents how close the patches are to interacting:

$$\phi(\mathbf{r}, \{\mathbf{p}\}) = \max_{\mathbf{p} \in \{\mathbf{p}\}} \hat{\mathbf{r}} \cdot \hat{\mathbf{p}} - \cos(\theta_m). \tag{8}$$

The function $\phi(\mathbf{r_{ij}}, \{\mathbf{p}_i\})$ is less than 0 if there is no patch on particle $i$ pointing in the direction of particle $j$, and larger than 0 if there is one. Two particles can only bond if $\phi_i(t) = \phi(\mathbf{r_{ij}(t)}, \{\mathbf{p}_i(t)\}) > 0$ and $\phi_j = \phi(\mathbf{r_{ji}(t)}, \{\mathbf{p}_j(t)\}) > 0$. If the two particles are already bonded, a possible bond breaking event will occur the first time either $\phi_i(t) = 0$ *or* $\phi_j(t) = 0$. If the particles are not bonded yet, a bonding event will take place the first time $\phi_i(t) = 0$ while $\phi_j(t) > 0$, or $\phi_j(t) = 0$ while $\phi_i(t) > 0$. Additionally, it is possible that the particles bond as soon as they enter each others interaction range; in that case, no numerical rootfinding is needed, and the bonding event can be handled immediately.

To find the points in time when $\phi = 0$, we use the numerical methods described in Ref. [3], solving the equation for each particle separately. In short, the value and derivative of $\phi(t)$ are calculated on a grid in time, and if the sign of $\phi$ changes between two grid points we know a solution to $\phi(t) = 0$ exists between those points. We then use Newton's method to find the event time. The derivatives are used to determine the possibility of grazing collisions, where $\phi(t)$ changes sign twice in the same interval. In this case, the derivative changes sign between two consecutive grid points, and a golden section search is used to find the extremum of the function. If the sign of $\phi(t)$ at the extremum is different than at the two nearest grid points, then Newton's method is used to find the root between the first grid point and the extremum.

If a well interaction event is found, it is added to the event tree, and the search is stopped. If the search reaches the end of the time interval where interactions can take place, the search is over as well, and a hard-core collision event is scheduled if $t_{\text{max}}$ corresponded to a core collision. Additionally, if the particles were bonded, a well escape event is scheduled when the distance between the two particles becomes larger than the maximum interaction range.

As it is likely that other collisions will prevent a patch binding event from happening if it is too far into the future, the search only extends for several searchsteps, after which a new event is scheduled to continue the search at a later time. Similarly, if two particles are unbonded and remain unbonded after both $\phi_i(t)$ and $\phi_j(t)$ have changed sign once, the remaining search is postponed until after the later of these two times.

### Patchy particle EDMD: event handling

There are three types of possible interaction events between patchy particles: hard-core collisions, well collisions, and well escapes. The hard-core collisions are handled exactly the same as those between hard spheres (see e.g. Ref. [2]). Both well escape and well collisions can happen in two ways: radially ($r = \sigma + \delta$), or laterally ($\phi_i = 0$ or $\phi_j = 0$). In case of radial bonding or escape, the well collisions and well escapes events are handled exactly the same as square well collision and escape events:

any forces involved are simply radial, and affect only the velocities (not the angular velocities) of the particles (see Ref. [2] for a full description).

The lateral well bonding and escape events are slightly more complicated. To handle these, we have to choose both the direction and location of the instantaneous forces applied to each particle, then modify the velocities and angular velocities of the particles while conserving total (kinetic plus potential) energy, momentum, and angular momentum. In particular, once the point of impact $\mathbf{r}_C$ and force direction $\hat{\mathbf{n}}$ are chosen, the velocity changes of the particles are given by:

$$\mathbf{v}_1^{\text{new}} = \mathbf{v}_1 + j\hat{\mathbf{n}}/m \quad (9)$$

$$\mathbf{v}_2^{\text{new}} = \mathbf{v}_2 - j\hat{\mathbf{n}}/m, \quad (10)$$

with $m$ the mass of a single particle, and $j$ a parameter determining the strength of the impulse $j\hat{\mathbf{n}}$. For the angular velocities:

$$\omega_1^{\text{new}} = \omega_1 + j(\mathbf{r}_C - \mathbf{r}_1) \times \hat{\mathbf{n}}/I \quad (11)$$

$$\omega_2^{\text{new}} = \omega_2 - j(\mathbf{r}_C - \mathbf{r}_2) \times \hat{\mathbf{n}}/I. \quad (12)$$

If the particle enters a well with well depth $\epsilon$, the collision parameter $j$ is given by:

$$j = \frac{-\mathbf{v}_C \cdot \hat{\mathbf{n}} - \sqrt{(\mathbf{v}_C \cdot \hat{\mathbf{n}})^2 + 2\epsilon A}}{A}, \quad (13)$$

with

$$\mathbf{v}_C = \mathbf{v}_1 - \mathbf{v}_2 + \boldsymbol{\omega_1} \times (\mathbf{r}_C - \mathbf{r}_1) - \boldsymbol{\omega_2} \times (\mathbf{r}_C - \mathbf{r}_2), \quad (14)$$

and

$$A = 2/m + ((\mathbf{r}_C - \mathbf{r}_1) \times \hat{\mathbf{n}})^2/I + ((\mathbf{r}_C - \mathbf{r}_2) \times \hat{\mathbf{n}})^2/I. \quad (15)$$

If the particle attempts to escapes the well, this will succeed only if $(\mathbf{v}_C \cdot \hat{\mathbf{n}})^2 - 2\epsilon A > 0$. In that case,

$$j = \frac{-\mathbf{v}_C \cdot \hat{\mathbf{n}} - \sqrt{(\mathbf{v}_C \cdot \hat{\mathbf{n}})^2 - 2\epsilon A}}{A}. \quad (16)$$

Otherwise, the particles will remain connected, and will bounce back, with:

$$j = \frac{-\mathbf{v}_C \cdot \hat{\mathbf{n}}}{A}. \quad (17)$$

Note that in principle, these events are not symmetric: only one of $\phi_i(t)$ and $\phi_j(t)$ is zero at the time of collision. We will call the particle for which this is true $p_1$, and the other $p_2$. The orientation of $p_2$ plays no role in this collision: only its center-of-of mass position has any influence on $\phi_1(t)$. Thus, the collision should not affect $p_2$'s angular momentum. Since the force between the particles is not radial, the only way to make sure no torque is exerted on $p_2$ is to apply the force to the center of mass of $p_2$: $\mathbf{r}_C = \mathbf{r}_2$. The direction of the impulse should be perpendicular to the cone describing the patch of $p_1$:

$$\mathbf{n} = \mathbf{p} - \frac{\mathbf{p} \cdot \mathbf{r}_{12}}{\mathbf{r}_{12} \cdot \mathbf{r}_{12}} \mathbf{r}_{12} \quad (18)$$

$$\hat{\mathbf{n}} = \frac{\mathbf{n}}{\sqrt{\mathbf{n} \cdot \mathbf{n}}}, \quad (19)$$

with $\mathbf{p}$ a vector pointing from the center of particle $p_1$ in the direction of the patch on $p_1$ that is interacting with $p_2$.

### Kern-Frenkel with a single bond per patch

To implement the single-bond-per-patch version of the Kern-Frenkel model in our EDMD simulations, we introduce a new event-type that essentially performs the Monte Carlo move we use for changing the bonds in the Monte Carlo simulations. We schedule an event that re-evaluates the bond of a randomly chosen patch according to equations (2) and (3). After handling the event, it is rescheduled at a later time. The interval between events is drawn from an exponential distribution corresponding to a fixed bond switching rate $\gamma$ for each patch. In other words, each patch will experience $\gamma\tau$ bond switching events every unit of time $\tau$.

Additionally, the change in potential energy for well collisions and well escape events is now always 0, as bonds are only made or broken during the bond-switching moves. As a result, the movement of the particles is unaffected. However, if a well escape event occurs for two bonded particles, the two particles will always remain connected, using equation (17) to calculate the collision parameter $j$. Note that the kinetic energy of the system is a conserved quantity if no thermostat is used.

## THERMODYNAMIC INTEGRATION

The thermodynamic integration paths used in this work are mostly standard.[4] When using the hard-sphere fluid or crystal as a reference state, it is important to note that our model only reduces to the HS model at $\epsilon/k_BT = -\infty$. Thus, the thermodynamic integration over the well depth (at fixed temperature) is given by:

$$\beta F_(\epsilon, \rho) = \beta F_{\text{HS}}(\rho) + \int_{-\infty}^{\epsilon} \mathrm{d}\epsilon' \left\langle \frac{\partial \beta U}{\partial \epsilon'} \right\rangle_{\epsilon'}. \quad (20)$$

Here, $F_(\epsilon, \rho)$ denotes the Helmholtz free energy at for well depth $\epsilon$ and density $\rho$, $F_{\text{HS}}(\rho)$ is the reference hard sphere free energy at density $\rho$ (calculated using the equation of state by Speedy [5]), $U$ is the potential energy of the system, and the thermodynamic average, indicated by $\langle . \rangle_{\epsilon'}$ is measured at interaction strength $\epsilon'$.

When applying the Frenkel-Ladd method to fluid configurations, we extract the positions and orientations of the particles from a fully bonded configuration obtained from an $NVT$ simulation at low $T$. To reduce the maximum spring constant required in the integration, it is helpful to make sure that no particles are close to either overlapping or breaking a bond. To do this, we first perform a short MC simulation biased towards configurations where no bonds are close to breaking, and no particles are close to overlapping. We then use a configuration from this simulation as the lattice positions and orientations for the Frenkel-Ladd method, resulting in the vibrational entropy of the configuration. During both the biased MC simulation and the thermodynamic integration, no bonds are allowed to break.

### Temperature dependence of the potential energy

The exponential decay of the number of broken bonds can be understood by examining the free energy of the liquid in the low-temperature liquid. In the limit of low temperatures, the number of broken bonds in the system becomes small, and it becomes reasonable to assume that these defects do not interact. For the disordered FCC and fluid phases at these patch widths, broken bonds can be seen to seperate into two defects, as the dangling bonds can diffuse through the system via bond switching. From this, we can estimate that the Helmholtz free energy $F$ as a function of the number of broken bonds $n_\mathrm{b}$ will behave as:

$$\beta F(n_\mathrm{b}) = \beta U - S/k_B \tag{21}$$

$$= \beta F(0) + n_\mathrm{b}\beta\epsilon - n_\mathrm{b}c - \log\binom{2n_\mathrm{b}}{4N}, \tag{22}$$

with $\beta = 1/k_BT$ the inverse temperature. In other words, breaking a bond is associated with an increase of the potential energy $\epsilon$, and a constant local increase in entropy $c$, due to the additional freedom of motion for the particles with a dangling bond. Additionally, the $2n_\mathrm{b}$ dangling bonds are distributed over $4N$ patches in total, leading to an addition entropic contribution analogous to mixing entropy. Writing the free energy instead as a function of the defect concentration $\alpha_{bb} = n_\mathrm{b}/N$, and taking the limit of small defect concentrations, we obtain:

$$\frac{\beta F(\alpha_{bb})}{N} = \frac{\beta F(0)}{N} - (2-\alpha_{bb})\beta\epsilon - \alpha_{bb}c - \frac{1}{N}\log\frac{(4N)!}{(2n_\mathrm{def})!(4N-2n_\mathrm{def})!}$$

$$\simeq \frac{\beta F(0)}{N} - (2-\alpha_{bb})\beta\epsilon + 2\alpha_{bb}\log\frac{\alpha_{bb}}{2} - \alpha_{bb} \tag{23}$$

Minimizing this free energy with respect to $\alpha_{bb}$, we obtain:

$$\alpha_{bb} = 2\exp(c/2 - 1)\exp(-\epsilon/2), \tag{24}$$

in close agreement with the measured potential energies in the disordered FCC and fluid phases. Interestingly, for the nearly fully bonded BCC and diamond phases, as well as the ordered FCC phase, broken bonds are typically not seen to split into two separated dangling bonds, as there is one specific bonding partner for each patch, as determined by the crystal structure. As a result, breaking a bond leads to only a single defect, and the number of broken bonds simply scales according to $\alpha_{bb} \propto \exp(-\beta\epsilon)$.

### Role of the switching rate on the diffusion coefficient

In the present model the bond switching rate $\gamma$ is an independent parameter. The dynamics is affected by the value of $\gamma$ only for $\gamma \ll 100\,\tau^{-1}$, as confirmed by the calculated dependence of $D$ on $\gamma$ shown in Fig. 1b. For low $\gamma$ , the diffusion constant is simply proportional to the bond-switching rate, as expected when the microscopic dynamics is slaved by the bond breaking and switching process. When the time it takes for two newly unbonded particles to move apart becomes significantly larger than $\gamma^{-1}$, $D$ becomes independent of $\gamma$, as multiple bond switching attempts on the same bond do not have any effect on the bonding probability. Interestingly, this indicates that the diffusion coefficient decays exponentially as a function of $\beta\epsilon$ (i.e. follows an Arrhenius law) not only at constant $\gamma\tau$, but also when the bond switching itself is a thermally activated process (such that $\gamma\tau \propto \exp(-\beta\epsilon_\gamma)$ for a constant activation energy $\epsilon_\gamma$).

An interesting analogue can be drawn to the recently reported vitrimers, a malleable plastic consisting of a mixture of organic polymerizered monomers, where a cat-

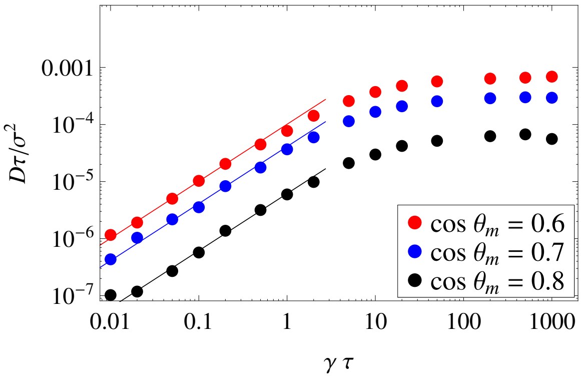


FIG. 1: Diffusion coefficients $D\tau/\sigma^2$ as a function of the inverse temperature $\beta\epsilon$, at constant bond switching rate $\gamma\tau = 100$, where $\tau = \sqrt{m\sigma^2/k_BT}$ is the time unit in the EDMD The solid lines are fits with slope -1/2, and the dashed line has slope -2. **b)** The diffusion coefficient as a function of the bond switching rate $\gamma\tau$, at constant temperature $k_BT/\epsilon = 0.1$. The lines are fits with slope 1.

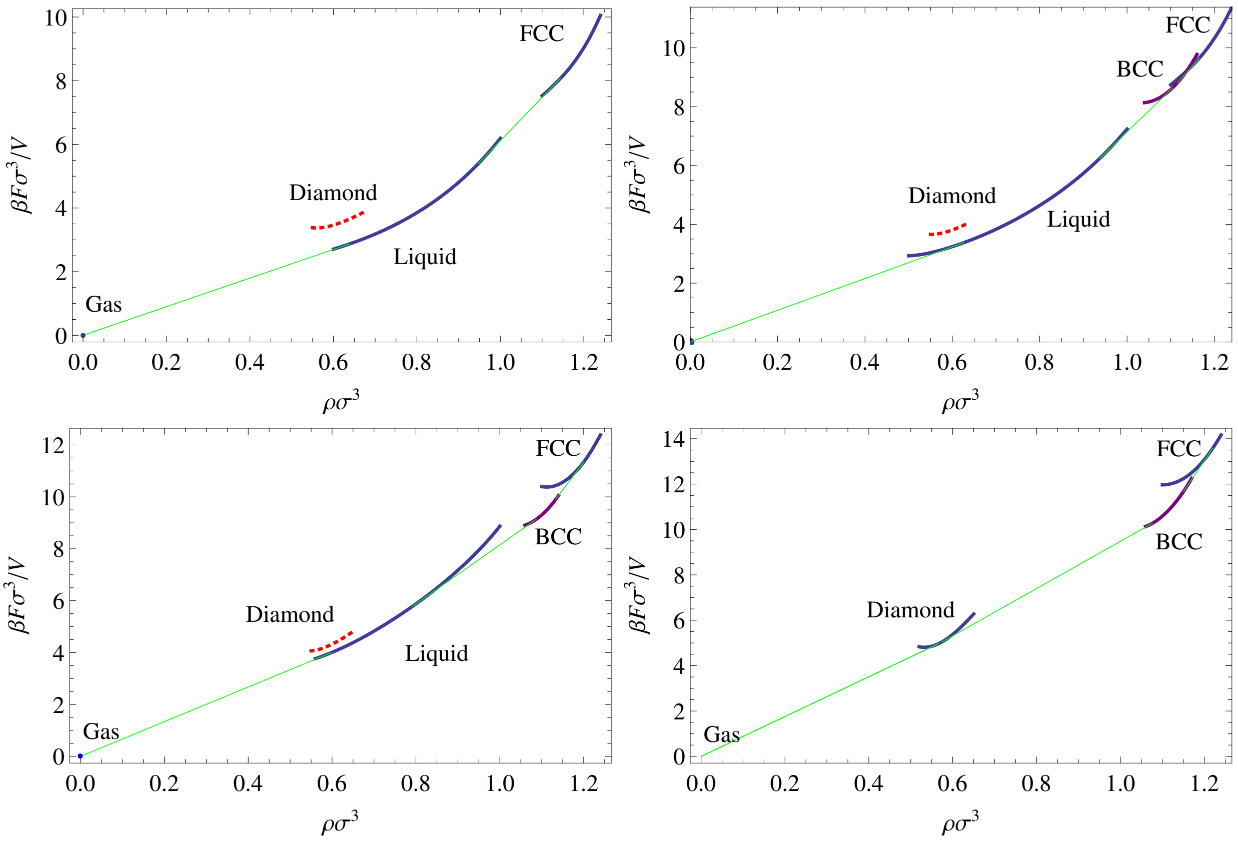


FIG. 2: Common tangents in the zero-temperature limit, for patch widths $\cos\theta_m = 0.6$ (top left), 0.7 (top right), 0.8 (bottom left) and 0.9 (bottom right). The green lines denote the common tangents. Only the phases where the free energy could be reliably calculated are shown.

alyst enables the switching (transesterification) of bonds between nearby bonding candidates[6]. Similar to the model system under consideration here, these vitrimers show an Arrhenius-like decay of the dynamics (in this case the viscosity) as a function of the temperature. Interestingly, the bond switching rate in our model can be linked to the amount of catalyst in the vitrimer system.


[1] N. Kern and D. Frenkel, J. Chem. Phys. **118**, 9882 (2003).

[2] D. C. Rapaport, Prog. Theor. Phys. Supp. **178**, 5 (2009).

[3] L. H. de la Peña, R. van Zon, J. Schofield, and S. B. Opps, J. Chem. Phys **126**, 074105 (2007).

[4] D. Frenkel and B. Smit, *Understanding Molecular Simulations: From Algorithms to Applications* (Academic Press, San Diego, 2002).

[5] R. J. Speedy, Journal of Physics: Condensed Matter **9**, 8591 (1997).

[6] D. Montarnal, M. Capelot, F. Tournilhac, and L. Leibler, Science **334**, (2011).
